# Supplementary material for: Dynamic swarms regulate the morphology and distribution of soft membrane domains
Source: arXiv:2402.06518 ancillary file (2024-06-11)
Supplement: Supplementary file 1 [file SI_Arnold_Gubbala_Takatori.pdf]

## SUPPLEMENTAL MATERIAL:

### Dynamic swarms regulate the morphology and distribution of soft membrane domains

Aakanksha Gubbala,<sup>\*</sup> Daniel P. Arnold,<sup>\*</sup> Anika Jena, Stephanie Anujararat, and Sho C. Takatori<sup>†</sup>  
*Department of Chemical Engineering, University of California, Santa Barbara, Santa Barbara, CA 93106*

#### CONTENTS

|                                                         |   |
|---------------------------------------------------------|---|
| I. Video Descriptions                                   | 2 |
| II. Detailed Experimental Methods                       | 2 |
| A. Buffers                                              | 2 |
| B. Actin and myosin preparation                         | 3 |
| C. Giant unilamellar vesicle (GUV) preparation          | 3 |
| D. Surface preparation                                  | 3 |
| E. Adsorbing a planar lipid bilayer to actin and myosin | 3 |
| F. Microscope for all imaging experiments               | 4 |
| G. Imaging passive lipid domains                        | 4 |
| H. Imaging active lipid domains                         | 4 |
| III. Image Analysis                                     | 4 |
| A. Intermediate scattering function calculations        | 4 |
| 1. Monte Carlo simulation of full domain relaxation     | 5 |
| B. Interfacial fluctuation analysis                     | 5 |
| IV. Theory                                              | 6 |
| A. Intermediate scattering function                     | 6 |
| B. Height fluctuations                                  | 7 |
| V. Simulation                                           | 8 |
| A. Numerical Details                                    | 8 |
| B. Mapping simulation parameters to physical properties | 9 |
| VI. Supplemental Figures                                | 9 |
| References                                              | 9 |

---

<sup>\*</sup> These authors contributed equally to this work

<sup>†</sup> stakatori@ucsb.edu

## I. VIDEO DESCRIPTIONS

**Video S1:** Experimental realization of complex active flows. (*Upper left*) Fluorescence micrographs show a two-phase lipid bilayer with liquid-ordered (Lo, green) domains in a liquid-disordered (Ld, black) continuous phase that evolves when in contact with active flows driven by heavy meromyosin (HMM) and actin. (*Upper right*) Actin filaments glide over a glass coverslip surface, driven laterally by HMM. Filaments align to form flocks, which preferentially associate with the Ld phase of the adsorbed bilayer. (*Lower*) Composite image containing actin (magenta) and Lo domains. Scale bar is 5  $\mu\text{m}$ .

**Video S2:** Passive experimental liquid-ordered (Lo) lipid membrane domain structural evolution. Fluorescence micrographs show a lipid bilayer with no actin and thus no active flows present. Lo domains (green) coarsen relatively slowly over time within a liquid-disordered (black) continuous phase. Heterogeneity in the apparent fluidity and Brownian motion of lipid domains suggests kinetic arrest due to friction with the underlying glass substrate. Scale bar is 5  $\mu\text{m}$ .

**Video S3:** Numerical solutions of the vorticity (*left*) and phase field (*right*) obtained from the Cahn-Hilliard–Toner-Tu equations. The model parameters are  $(M, \kappa, \Gamma_0, \Gamma_2, \alpha, \beta, S) = (1, 0.25, -1, 1, -0.2, 1, 1)$ .

**Video S4:** Numerical solutions of the vorticity (*left*) and phase field (*right*) obtained from the Cahn-Hilliard–Toner-Tu equations. The model parameters are  $(M, \kappa, \Gamma_0, \Gamma_2, \alpha, \beta, S) = (1, 0.25, -1, 1, -0.2, 1, 7)$ .

**Video S5:** Evolution of an initially circular domain under swarming flows. Numerical simulations of the coupled Cahn-Hilliard–Toner-Tu equations for  $S = 1$  (*left*) and  $S = 7$  (*right*). The rest of the model parameters are  $(M, \kappa, \Gamma_0, \Gamma_2, \alpha, \beta) = (1, 0.25, -1, 1, -0.2, 1)$ .

**Video S6:** Two realizations of active liquid-ordered (Lo) lipid membrane domains with prominent interfacial fluctuation. (*Left column*) Fluorescence micrographs show a two-phase lipid bilayer with a single Lo domain (green) in a liquid-disordered (Ld, black) continuous phase. With active flows present, the quasi-1D interface between the Lo and Ld phases undergoes significant low-frequency oscillations. (*Right column*) Flocks of actin filaments gliding near the lipid bilayer induce membrane flows that perturb the quasi-1D domain boundaries. Scale bar is 2  $\mu\text{m}$ .

**Video S7:** A liquid-ordered (Lo) lipid membrane domain undergoes fission and pinch-off while being advected by actin flows. (*Left*) An approximately-circular Lo domain encounters actin flows, beginning at time  $t = 0\text{s}$ . Actin flows quickly cause a small domain to pinch off of the membrane, before a fusion occurs, causing the remaining domain to split approximately in half. In the frames leading up to this fission event, significant deformations appear in the domain interface, causing the radius  $R(\theta, t)$  to take on multiple values for a given  $\theta$ . This makes the height fluctuation analysis, including the Fourier transform, discussed in Fig. S3 impossible. (*Right*) Actin flows are triggered at time  $t = 0\text{ s}$ , causing swarms to form and move across the region of interest over time.

**Video S8:** A passive liquid-ordered (Lo) lipid membrane domain evolves over time, in the absence of active flows. Interfacial fluctuations are restricted primarily to higher frequencies. Scale bar is 2  $\mu\text{m}$ .

## II. DETAILED EXPERIMENTAL METHODS

### A. Buffers

Filamentous actin buffer (F-buffer) consists of 50 mM Tris (pH 7.5), 2 mM magnesium chloride, 0.5 mM adenosine triphosphate (ATP), 0.2 mM calcium chloride, 25 mM potassium chloride, and 1 mM dithiothreitol (DTT). DTT is added to all buffers immediately before use to preserve its reactivity.

Assay buffer (A-buffer) consists of 25 mM imidazole (pH 7.4), 4 mM magnesium chloride, 1 mM (ethylene glycol-bis( $\beta$ -aminoethyl ether)-N,N,N',N'-tetraacetic acid) (EGTA), 25 mM potassium chloride, and 1 mM DTT.

Globular actin buffer (G-buffer) consists of 2 mM Tris (pH 8.0), 0.2 mM calcium chloride, 0.5 mM DTT, 1 mM sodium azide, and 0.2 mM ATP.

## B. Actin and myosin preparation

Rabbit skeletal muscle actin is purified from muscle acetone powder (Pel-Freez, catalog no: 41995-2, Lot 16743) using standard methods [1, 2]. No rabbits or other animals are directly involved in this study. Actin is stored as depolymerized globular actin (G-actin) at  $-80^{\circ}\text{C}$  in G-buffer with 6% sucrose until use.

Actin is labeled with fluorescent Alexa Fluor 555 NHS Ester (Succinimidyl Ester) (Invitrogen catalog no: A20009) for microscopic visualization. G-actin is reacted with NHS-Alexa Fluor 555 in HEPES buffer at room temperature for 30 minutes. 2x-concentrated F-buffer is then added to the G-actin, quenching the NHS reaction and causing G-actin to polymerize to F-actin. F-actin polymerization proceeded for 30 minutes at room temperature, and then overnight at  $4^{\circ}\text{C}$ . Labeled F-actin is centrifuged at  $142,000 \times g$  for 30 minutes, and the pellet collected. Unreacted dye and defective G-actin monomers and oligomers that are unable to polymerize are discarded in the supernatant. Labeled F-actin is dissolved in G-buffer, and allowed to de-polymerize for three days at  $4^{\circ}\text{C}$  before freezing and storing in 6% sucrose at  $-80^{\circ}\text{C}$ .

Heavy meromyosin (HMM) is purified from rabbit skeletal muscle (Pel-Freez Biologicals, Rogers, Arkansas) using standard methods [3]. HMM is frozen in 10 mM potassium phosphate buffer (pH 7.0), 100 mM potassium chloride, 0.3 mM EGTA, 1 mM DTT, and 6% sucrose at  $-80^{\circ}\text{C}$  until use.

## C. Giant unilamellar vesicle (GUV) preparation

Giant unilamellar vesicles (GUVs) are prepared using the established electroformation method [4]. Briefly, lipids are mixed with the following composition: 44.7% 1,2-dioleoyl-sn-glycero-3-phosphocholine (DOPC, Avanti catalog no: 850375P), 34.7% 1,2-dipalmitoyl-sn-glycero-3-phosphocholine (DPPC, Avanti catalog no: 850355C), 15% cholesterol (TCI Chemical, catalog no: C3624), 5% 1,2-dioleoyl-3-trimethylammonium-propane (DOTAP, Avanti catalog no: 890890P), 0.3% 1,2-distearoyl-sn-glycero-3-phosphoethanolamine-N-[poly(ethylene glycol)2000-N'-carboxyfluorescein] (DSPE-PEG2k-FITC, Avanti catalog no: 810120C), and 0.3% ATTO 647-labeled 1,2-dioleoyl-sn-glycero-3-phosphoethanolamine (ATTO 647-DOPE, ATTO-TEC catalog no: AD 647-161). This mixture of lipids and cholesterol phase-separates into liquid-ordered (Lo) domains dispersed within a liquid-disordered (Ld) continuous phase. Lipids are spread on an indium tin oxide (ITO)-coated microscope slide (Diamond Coatings, 8-12 Ohm slide) and dried under vacuum for 30 minutes.

A 2 mm rubber gasket is sandwiched between the ITO-coated slide containing lipids and a clean ITO-coated slide, and the interstitial space filled with 75 mM sucrose solution. A sinusoidal electric potential of amplitude 3V (peak-to-peak) and frequency 10 Hz is applied to the chamber for one hour at  $50^{\circ}\text{C}$ . After one hour, the frequency is changed to 2 Hz for 30 minutes. The resulting GUVs are collected, stored at room temperature and used within one day.

## D. Surface preparation

Glass cover slips No. 1.5 (Azer Scientific) are cleaned with piranha solution (3:1 sulfuric acid:hydrogen peroxide) for five minutes and then washed with deionized water. The cover slips are then made hydrophobic via reaction with trimethylchlorosilane (Sigma-Aldrich) vapors in a vacuum chamber, under house vacuum for ten minutes. A 6 mm cylindrical polydimethylsiloxane (PDMS) chamber is attached to the cover slip surface to hold liquids.

Cover slips are incubated with 200 nM heavy meromyosin (HMM) for ten minutes. Free, un-adsorbed HMM is then washed away with A-buffer. Active samples are then incubated in 1  $\mu\text{M}$  Alexa Fluor 555-labeled F-actin for 5 minutes, while passive samples did not contain actin and sample preparation proceeded according to Section II E. Unbound actin is washed away with A-buffer. Finally, the actomyosin-treated surface is washed with MilliQ water, to remove salts and promote bilayer adhesion.

## E. Adsorbing a planar lipid bilayer to actin and myosin

For active samples, GUVs in MilliQ water are added to the actin/HMM-coated cover slip surface. For passive samples, actin is not used and GUVs are directly adsorbed to an HMM-coated cover slip. The cover slip is heated to  $37^{\circ}\text{C}$  for at least 20 minutes, during which time GUVs rupture on the treated surface, presumably due to electrostatic attraction between positively-charged DOTAP lipids and negatively-charged glass. Unbound GUVs are then washed from the cover slip with A-buffer.

## F. Microscope for all imaging experiments

All imaging is carried out on an inverted Nikon Ti2-Eclipse microscope (Nikon Instruments) using an oil-immersion objective (Apo 100x, NA 1.45, oil). Lumencor SpectraX Multi-Line LED Light Source is used for excitation (Lumencor, Inc). Fluorescent light is spectrally filtered with emission filters (432/36, 515/30, 595/31, and 680/42; Semrock, IDEX Health and Science) and imaged on a Photometrics Prime 95 CMOS Camera (Teledyne Photometrics). Microscope images are collected using MicroManager 1.4 software [5].

## G. Imaging passive lipid domains

Planar lipid membranes without actin are kept in A-buffer at room temperature for approximately 10 minutes before imaging. Thus, lipid domains are given time to coarsen to approximately 5  $\mu\text{m}$  in size. Membranes are imaged for 450-600 s at room temperature, with 2-5 s time intervals to observe passive domain behavior.

## H. Imaging active lipid domains

Planar lipid membranes adsorbed to actin and HMM are kept in A-buffer at room temperature for approximately 10 minutes before imaging, allowing them to coarsen to several microns in size. Photosensitive caged ATP (1 $\mu\text{M}$  DMNPE-caged ATP, Invitrogen catalog no: A1049) is added to planar lipid membranes with actin and myosin before imaging. Bilayer/actin samples are irradiated with a brief (<1 s) pulse of 404 nm light, converting the caged ATP to usable ATP and triggering actin flows. Lipid domains are imaged at 2-second intervals as actin flows interacted with them. Imaging continued for 40-80 s, until actin motion largely ceased, possibly due to friction between actin bundles and the membrane, or ATP transport limitations.

# III. IMAGE ANALYSIS

## A. Intermediate scattering function calculations

Microscope images of lipid domains are thresholded in ImageJ to create binary images. While not strictly necessary for analysis of lipid domain structure, we find binarizing the images to be the most effective way to eliminate artifacts resulting from FITC photo-bleaching during long time-lapses. It is also necessary to use binary images for the simulations discussed in Section III A 1.

The intermediate scattering function is calculated using similar methodology to differential dynamic microscopy (DDM) microrheology measurements [6, 7]. The difference in pixel intensity  $\Delta I(\mathbf{x}; t)$  is calculated at all positions  $\mathbf{x}$ , between pairs images of the same sample separated by lag time  $t$  [Supplemental Fig. S1(a)]:

$$\Delta I(\mathbf{x}, t) = I(\mathbf{x}, t) - I(\mathbf{x}, 0). \quad (1)$$

The Fourier transform of intensity differences with respect to position is defined as  $\Delta \hat{I}(\mathbf{k}; t) = 1/(2\pi) \int \Delta I(\mathbf{x}; t) e^{-i\mathbf{k} \cdot \mathbf{x}} d\mathbf{x}$  and taken using the fast Fourier transform (FFT) method [Fig. S1(b)]. The image structure function  $D(\mathbf{k}, t)$  is defined as

$$D(\mathbf{k}, t) = \langle |\Delta \hat{I}(\mathbf{k}, t)|^2 \rangle \quad (2)$$

where  $\langle \cdot \rangle$  denotes an ensemble average of all differences in pairs of images separated by a particular lag time  $t$ . Values of  $\Delta \hat{I}(\mathbf{k}; t)$  from the FFT output matrix are also binned into shells of width  $\approx 0.5 \mu\text{m}^{-1}$ , and averaged [Supplemental Fig. S1(c),(d)]. Thus it is appropriate to write  $D(k, t)$  where  $k = |\mathbf{k}|$ .

The structure function  $D(k, t)$  is related to the intermediate scattering function  $F(k, t)$ , by

$$D(k, t) = A(k) [1 - F(k, t)] + B(k). \quad (3)$$

In DDM microrheology analysis,  $A(k)$  represents a wave vector-dependent constant related to the scattering properties of particles and  $B(k)$  represents camera noise [8]. For diffusive scatterers without flow,  $F(k, t)$  is expected to decay according to  $F(k, t) = e^{-\alpha(k)t}$ , where  $1/\alpha(k)$  is the relaxation time. Thus, for a DDM dataset with many relaxations, it is possible to find  $A(k)$  and  $B(k)$  using the asymptotic behavior  $F(k, t \rightarrow 0) = 1$  and  $F(k, t \rightarrow \infty) = 0$ , as these

asymptotes give  $D(k, t \rightarrow \infty) = A(k) + B(k)$  and  $D(k, t \rightarrow 0) = B(k)$ . However, without having experimental access to multiple domain relaxations, it is impossible to accurately estimate  $D(k, t \rightarrow \infty)$ . Moreover, our active Fig. 2 of the main text does not follow an exponential profile. Thus, a three-parameter nonlinear fit is prone to significant error and should not be used.

To find  $A(k)$  and  $B(k)$ , we conduct simulations to predict the fully relaxed domain configuration, thus estimating  $D(k, t \rightarrow \infty)$ . We generate a series of random configurations using Monte Carlo methods, as described in Section III A 1. Differences between all pairwise combinations of 30 simulated domain conformations are sampled, yielding  $\binom{30}{2} = 435$  independent data sets of  $\Delta I(\mathbf{k}, t)$ . After applying Eq. 2 to find the image structure function  $D(k, t)$ , we take an average  $\langle \cdot \rangle$  of the 435 samples to obtain

$$C(k) = \langle D(k, t \rightarrow \infty) \rangle = A(k) + B(k). \quad (4)$$

Finally, to find  $B(k)$ , we simply consider the short-time behavior of the domains without simulations:

$$B(k) = D(k, t \rightarrow 0) \quad (5)$$

and take  $B(k)$  to be the value of  $D(k, t)$  at the earliest nonzero time point sampled. The process for generating  $C(k)$  from simulation data is described graphically in Supplemental Fig. S2.

Thus we use  $B(k)$  and our simulated  $C(k)$  to find the intermediate scattering function [Supplemental Fig. S1(e)]:

$$F(k, t) = 1 - \frac{D(k, t) - B(k)}{C(k) - B(k)}. \quad (6)$$

### 1. Monte Carlo simulation of full domain relaxation

To find the image structure function of fully relaxed lipid domains,  $\Delta \hat{I}(\mathbf{k}, t \rightarrow \infty)$  we use Monte Carlo simulations to scramble the domain configuration at the final time point of each experimental data set.

From the binary image at the final time point of a given experiment, we identify distinct black and white objects (domains) and measure their areas [Supplemental Fig. S2(a)]. To simulate new domain configurations, we assume that domains are circular and do not change size as the system evolves. In our active experiments we do observe many non-circular domains, over the longer time scales of passive experiments, we do observe some coarsening and a small increase in overall domain size.

We then construct a new black and white image containing circles with areas matching those of the domains in the original image [Supplemental Fig. S2(b)]. Circles are randomly placed, one at a time, subject to a hard circle interaction potential between domains. Thus, if a domain is randomly placed such that it overlaps with a previously-placed domain, then the improperly-placed domain will continue to sample random positions until it does not touch any other domains. It should be noted that periodic boundary conditions are not imposed, and domains may straddle the edge of the simulation window. The part of any domain lying outside the simulation boundaries is ignored in subsequent structure calculations. This is consistent with the experimental data, in which parts of domains lying outside the field of view are ignored. Domain placement proceeds until all domains have been randomly placed in the simulation window.

The simulation is repeated 30 times for each experiment. Differences between all distinct pairs of 30 realizations are taken according to Eq. 1 to give

$$C(\mathbf{k}) = \langle |\Delta \hat{I}(\mathbf{k}, t \rightarrow \infty)|^2 \rangle \quad (7)$$

where  $\langle \cdot \rangle$  denotes an ensemble average of all subtracted pairs (for 30 samples, there are 435 distinct pairs) [Supplemental Fig. S2(c)-(d)]. Wave vectors are subsequently binned and radially averaged as described in Section III A, yielding the  $C(k)$  that appears in Eq. 6 [Supplemental Fig. S2(e)].

## B. Interfacial fluctuation analysis

To quantify the fluctuations in the domain interfaces, we first use the Canny edge detection algorithm to trace the boundary of lipid domains in either experimental images or simulations [Supplemental Fig. S8(a)]. We remove extraneous edges outside the domain, and then find the center of mass of the domain. We calculate the distance  $R(\theta)$  between each point in the discretized edge and the center of mass, as a function of the azimuthal angle  $\theta$  [Supplemental Fig. S8(b)]. We find the radius of an equivalent circle by taking the mean of all radii, over all time points for given

domain:  $R_0 = \langle R(\theta) \rangle_{\theta,t}$ . Experimental interfacial height data is measured over relatively short time windows ( $<12$  s), with domains that undergo visible fission or fusion excluded. Thus we assume that domain size is approximately constant during this time. We define the “height” of the interface as the difference between the local radius and mean radius, replacing  $\theta$  with an effective arc length  $s = R_0\theta$  [Supplemental Fig. S8(b),(c)]

$$h(s, t) = R(s, t) - R_0. \quad (8)$$

We take the discrete Fourier transform of  $\hat{h}(k, t) = \mathcal{F}_s \{h(s, t)\}$  with respect to arc length  $s = R_0\theta$  [Fig. S8(d)]. In Supplemental Fig. S9, we plot the magnitude  $|\hat{h}(k, t)|$  of these height fluctuations. For passive experiments we take the mean of 14 independent lipid domains. For simulations, we consider four replicate runs. For active experiments, we plot three individual trajectories.

#### IV. THEORY

We use the Cahn-Hilliard equation [9] to study the evolution of multi-phase lipid domains. It is given by

$$\partial_t \phi(\mathbf{x}, t) + \mathbf{v} \cdot \nabla \phi = M \nabla^2 \mu, \quad \mu = \phi^3 - \phi - \kappa \nabla^2 \phi, \quad (9)$$

where  $\phi$  is the order parameter for lipid concentration,  $\mathbf{v}$  is the velocity,  $M$  is the lipid mobility, and  $\kappa$  is a surface tension parameter. The domain structure is affected by swarming actin filaments. We model this swarming flow by using the Toner-Tu equation [10], given by

$$\partial_t \mathbf{v}(\mathbf{x}, t) + (1 - S) \mathbf{v} \cdot \nabla \mathbf{v} = -\frac{S}{2} \nabla |\mathbf{v}|^2 - \nabla P + \Gamma_0 \nabla^2 \mathbf{v} - \Gamma_2 \nabla^4 \mathbf{v} - (\alpha + \beta |\mathbf{v}|^2) \mathbf{v} - \phi \nabla \mu, \quad (10)$$

where the parameters are described in the main text. Note that the equations are two-way coupled –  $\phi$  is advected by  $\mathbf{v}$  generated from the Toner-Tu model and  $\mathbf{v}$  in turn is influenced by  $\phi$  through the body force term  $\phi \nabla \mu$ . To understand the effect of the body force term on domain structure, we performed numerical simulations with the body force term, denoted by ‘two-way coupling’, and without the body force term, denoted by ‘one-way coupling’. In Fig. S3, we see that the domains have sharper edges in the one-way coupling case, while the domains in the two-way coupling case are smoother and elongated. The Toner Tu flows respond to gradients in chemical potential and evolve to denser flocks that lead enhanced mixing of domains.

With the two-way coupled Cahn-Hilliard–Toner-Tu equations, we first examine the steady state morphology of domains by deriving an equation for the intermediate scattering function. Second, we derive an equation for interfacial height to analyse the initial instabilities at the interface of the domain.

##### A. Intermediate scattering function

The intermediate scattering function  $F(k, t)$  is defined as

$$F(k, t) = \frac{\langle \hat{\phi}(\mathbf{k}, t) \hat{\phi}(-\mathbf{k}, 0) \rangle_t}{\langle |\hat{\phi}(\mathbf{k}, 0)|^2 \rangle} \quad (11)$$

where  $\hat{\phi}(k, t) = \mathcal{F}_{\mathbf{x}} \{\phi(\mathbf{x}, t)\}$ , the brackets  $\langle \cdot \rangle_t$  denotes a time correlation, and  $k = |\mathbf{k}|$  is the radially averaged wave number. To get an evolution equation for  $F(k, t)$ , we first Fourier transform Eq. 9:

$$\partial_t \hat{\phi}(\mathbf{k}, t) + \mathcal{F}_{\mathbf{x}} \{\mathbf{v} \cdot \nabla \phi\} = -Mk^2(\kappa k^2 - 1) \hat{\phi} - Mk^2 \mathcal{F}_{\mathbf{x}} \{\phi^3\}. \quad (12)$$

Next, we multiply Eq. 12 by  $\hat{\phi}(-\mathbf{k}, 0)/\langle |\hat{\phi}(\mathbf{k}, 0)|^2 \rangle$  and take  $\langle \cdot \rangle$  to get

$$\partial_t F(k, t) + V(k, t) = -\frac{F}{\tau_p(k)} - Mk^2 N(k, t), \quad (13)$$

where  $\tau_p = (Mk^2(\kappa k^2 - 1))^{-1}$  is the passive relaxation time. The functions  $V(k, t)$  and  $N(k, t)$  in Eq. 13 are defined as

$$V(k, t) = \frac{\langle \mathcal{F}_{\mathbf{x}} \{\mathbf{v} \cdot \nabla \phi\} \hat{\phi}(-\mathbf{k}, 0) \rangle_t}{\langle |\hat{\phi}(\mathbf{k}, 0)|^2 \rangle} \quad \text{and} \quad N(k, t) = \frac{\langle \mathcal{F}_{\mathbf{x}} \{\phi^3\} \hat{\phi}(-\mathbf{k}, 0) \rangle_t}{\langle |\hat{\phi}(\mathbf{k}, 0)|^2 \rangle}. \quad (14)$$

We now focus on simplifying  $V(k, t)$ . Using the convolution theorem, we can compute the Fourier transform,  $\mathcal{F}_{\mathbf{x}}\{\mathbf{v} \cdot \nabla \phi\}$ , as

$$\mathcal{F}_{\mathbf{x}}\{\mathbf{v} \cdot \nabla \phi\} = i \int d\mathbf{q} \, \hat{\mathbf{v}}(\mathbf{k} - \mathbf{q}, t) \cdot \mathbf{q} \, \hat{\phi}(\mathbf{q}, t) . \quad (15)$$

The convolution introduces a coupling between the wave vectors  $\mathbf{k} - \mathbf{q}$  and  $\mathbf{q}$ . This form of coupling also arises in the equations in mode coupling theory [11]. Substituting this result in the expression for  $V(k, t)$  gives

$$V(k, t) = i \frac{1}{\langle |\hat{\phi}(\mathbf{k}, 0)|^2 \rangle} \left\langle \int d\mathbf{q} \, \hat{\mathbf{v}}(\mathbf{k} - \mathbf{q}, t) \cdot \mathbf{q} \, \hat{\phi}(\mathbf{q}, t) \hat{\phi}(-\mathbf{k}, 0) \right\rangle_t . \quad (16)$$

Within the bracket, multiply and divide by  $\hat{\phi}(\mathbf{k}, t)$  to get

$$V(k, t) = i \frac{1}{\langle |\hat{\phi}(\mathbf{k}, 0)|^2 \rangle} \left\langle \int d\mathbf{q} \, \hat{\mathbf{v}}(\mathbf{k} - \mathbf{q}, t) \cdot \mathbf{q} \frac{\hat{\phi}(\mathbf{q}, t)}{\hat{\phi}(\mathbf{k}, t)} \hat{\phi}(\mathbf{k}, t) \hat{\phi}(-\mathbf{k}, 0) \right\rangle_t . \quad (17)$$

We can split this four-term correlation into two two-term correlations:

$$V(k, t) = i \frac{\langle \hat{\phi}(\mathbf{k}, t) \hat{\phi}(-\mathbf{k}, 0) \rangle_t}{\langle |\hat{\phi}(\mathbf{k}, 0)|^2 \rangle} \left\langle \int d\mathbf{q} \, \hat{\mathbf{v}}(\mathbf{k} - \mathbf{q}, t) \cdot \mathbf{q} \frac{\hat{\phi}(\mathbf{q}, t)}{\hat{\phi}(\mathbf{k}, t)} \right\rangle_t . \quad (18)$$

It is convenient to define a new function,  $\Lambda(k, t)$ , given by

$$\Lambda(k, t) = \left\langle \int d\mathbf{q} \, \hat{\mathbf{v}}(\mathbf{k} - \mathbf{q}, t) \cdot \mathbf{q} \frac{\hat{\phi}(\mathbf{q}, t)}{\hat{\phi}(\mathbf{k}, t)} \right\rangle_t . \quad (19)$$

Using Eq. 19 and the definition of the intermediate scattering function from Eq. 11, we get

$$V(k, t) = i \Lambda(k, t) F(k, t) . \quad (20)$$

After substituting the function for  $V(k, t)$ , Eq. 13 becomes:

$$\partial_t F(k, t) = - \left( \frac{1}{\tau_p(k)} + i \Lambda(k, t) \right) F(k, t) - M k^2 N(k, t) . \quad (21)$$

The Toner Tu equations are analytically intractable so we end our analysis with Eq. 21. We note that Eq. 21 is a general equation for any evolving order parameter with flow. Furthermore, the solution to Eq. 21 is likely to be non-exponential. If we ignore the cubic non-linearity, the solution to Eq. 21 is given by

$$F(k, t) = e^{-\frac{t}{\tau_p(k)}} \times e^{-i \int_0^t \Lambda(k, t') dt'} . \quad (22)$$

The convective term in the Cahn-Hilliard equation predicts oscillatory behavior in the relaxation dynamics. Previously, oscillatory behavior has been observed for systems of Active Brownian Particles (ABPs) [12–14] and bacterial suspensions [15].

## B. Height fluctuations

We follow Bray's method [16] to derive an equation for interfacial height from the Cahn-Hilliard model. Consider a flat interface of a phase separated domain located at a height,  $h(x, t)$ . First, we transform the concentration phase field as  $\phi(x, y, t) = f(y - h(x, t))$ , where  $f$  is the Heaviside function. Now, we introduce a new variable,  $u = y - h(x, t)$ . We obtain the following derivatives of  $\phi$  in terms of  $f(u)$ :

$$\partial_t \phi = -f'(u) \partial_t h \quad (23a)$$

$$\nabla \phi = -f'(u) \partial_x h \mathbf{e}_x + f'(u) \mathbf{e}_y \quad (23b)$$

$$\nabla^2 \phi = f''(u) (1 + (\partial_x h)^2) - f'(u) \frac{\partial^2 h}{\partial x^2} . \quad (23c)$$

Substituting the relations in Eq. 23 in Eq. 9 gives

$$-f'(u)[\partial_t h + v_x \partial_x h - v_y] = M \nabla^2 \left( f^3 - f - \kappa \left( f''(u)(1 + (\partial_x h)^2) - f'(u) \frac{\partial^2 h}{\partial x^2} \right) \right), \quad (24)$$

where we decompose the velocity vector into its components as  $\mathbf{v} = v_x \mathbf{e}_x + v_y \mathbf{e}_y$ . We apply the inverse Laplacian operator  $(\nabla^2)^{-1}$  to Eq. 24 to give

$$(-\nabla^2)^{-1} f'(u)[\partial_t h + v_x \partial_x h - v_y] = M \left( f^3 - f - \kappa \left( f''(u)(1 + (\partial_x h)^2) - f'(u) \frac{\partial^2 h}{\partial x^2} \right) \right). \quad (25)$$

This operation eliminates fourth order derivatives. We now multiply Eq. 25 by  $f'(u)$  and integrate over  $u$  to give

$$\int_{-\infty}^{\infty} du f'(u) (-\nabla^2)^{-1} f'(u) [\partial_t h + v_x \partial_x h - v_y] = M \int_{-\infty}^{\infty} du f'(u) \left( f^3 - f - \kappa \left( f''(u)(1 + (\partial_x h)^2) - f'(u) \frac{\partial^2 h}{\partial x^2} \right) \right). \quad (26)$$

Note that  $f'(u)$  is a smeared  $\delta$  function. The strength of the  $\delta$  is proportional to concentration difference across the interface, given by  $\Delta\phi = 2$ . The integrals containing delta have a maxima at  $u = 0$ , simplifying integrals on the right as:

$$\int_{-\infty}^{\infty} du f'(u) (f^3 - f) = 0, \quad \int_{-\infty}^{\infty} du f'(u) f''(u) = 0. \quad (27)$$

Eq. 26 now becomes

$$\int_{-\infty}^{\infty} du f'(u) (-\nabla^2)^{-1} f'(u) [\partial_t h + v_x \partial_x h - v_y] = M \kappa \sigma \frac{\partial^2 h}{\partial x^2}, \quad (28)$$

where  $\sigma = \int_{-\infty}^{\infty} du [f'(u)]^2$  is the surface tension. From here, it is convenient to operate in the Fourier space. We define the Fourier transform in x-direction as  $\tilde{f} = \mathcal{F}_x\{f\}$ . Fourier transform of Eq. 28 gives

$$\int_{-\infty}^{\infty} du f'(u) \mathcal{F}_x\{(-\nabla^2)^{-1} f'(u) [\partial_t h + v_x \partial_x h - v_y]\} = -M \kappa \sigma k_x^2 \tilde{h}. \quad (29)$$

The Fourier transform of the inverse Laplacian operator, denoted as  $G(x, y) = (-\nabla^2)^{-1} F(x, y)$ , is given by

$$\tilde{G}(k_x, y) = \frac{1}{2k_x} \int_{-\infty}^{\infty} dy' e^{-k_x |y - y'|} \tilde{F}(k_x, y'). \quad (30)$$

We use the above identity in Eq. 29 to get

$$\frac{1}{2k_x} \int_{-\infty}^{\infty} \int_{-\infty}^{\infty} du dv e^{-k_x |u - v|} f'(u) f'(v) [\partial_t \tilde{h} + \mathcal{F}_x\{v_x \partial_x h\} - \tilde{v}_y] = -M \kappa \sigma k_x^2 \tilde{h}. \quad (31)$$

The integral on the left has a maxima at  $u = v = 0$ . After eliminating the integral, we are left with the final equation for interfacial height:

$$\partial_t \tilde{h}(k_x, t) + \mathcal{F}_x\{v_x \partial_x h\} = -\zeta(k_x) \tilde{h} + \tilde{v}_y(k_x, t), \quad (32)$$

where  $\zeta(k_x) = -1/2 M \kappa \sigma k_x^2$  is a drag factor. Eq. 32 is a general evolution equation for height spectra. It is analogous to the typical advection-diffusion-reaction equations encountered in engineering. The velocity normal to the interface ( $v_y$ ) modulates the growth of the perturbations, similar to a source or sink term.

## V. SIMULATION

### A. Numerical Details

A Fourier transform of Eqs. 9-10 gives a system of coupled first-order differential equations:

$$\frac{d\hat{\phi}}{dt} = -\mathcal{F}\{\mathbf{v} \cdot \nabla \phi\} - M k^2 \mathcal{F}\{\phi^3 - \phi\} - M \kappa k^4 \hat{\phi}, \quad (33)$$

$$\frac{d\hat{\omega}}{dt} = -(\Gamma_0 k^2 + \Gamma_2 k^4) \hat{\omega} - (1 - S) \mathcal{F}\{\mathbf{v} \cdot \nabla \omega\} - \mathcal{F}\{\nabla \times [(\alpha + \beta |\mathbf{v}|^2) \mathbf{v}]\} - \mathcal{F}\{\nabla \times (\phi \nabla \mu)\}. \quad (34)$$

Here,  $\omega = \nabla \times \mathbf{v}$  is the vorticity. By taking a curl to get vorticity, we eliminate the gradient terms in Eq. 10. The ODEs are solved using forward finite difference on a  $512 \times 512$  grid and implicitly treating  $\nabla^2$  and  $\nabla^4$  terms. To remove high frequency noise, a 2/3 anti-aliasing filter is applied to the five non-linear terms in Eqs. 33-34: bulk free energy ( $\phi^3 - \phi$ ), convection, flocking term  $((\alpha + \beta|\mathbf{v}|^2)\mathbf{v})$ , and body force ( $\phi\nabla\mu$ ). The time step is controlled with adaptive time stepping,  $\Delta t_{new} = [tol/|\phi(t; \Delta t) - \phi(t; \Delta t/2)|]^{1/5}$ . Here,  $\phi(t; \Delta t)$  means using a time step  $\Delta t$  to calculate  $\phi(t)$ , and the tolerance,  $tol$  is  $5 \times 10^{-4}$  for  $S = 1$  and  $10^{-3}$  for  $S = 7$ . The dimensions of the system are  $32\pi \times 32\pi$ . The initial system configuration is  $\phi = \phi_{avg} + 0.1 \times \text{noise}$ , where  $\phi_{avg} = 0.35$ . The initial vorticity is  $\omega = 10^{-3} \times \text{noise}$ .

## B. Mapping simulation parameters to physical properties

The total free energy,  $F[\phi]$  for a binary system is given by the Ginzburg-Landau expansion,

$$F[\phi(\mathbf{x}, t)] = \int d\mathbf{x} \left( \frac{b}{4}\phi^4 - \frac{a}{2}\phi^2 + \frac{\kappa}{2}|\nabla\phi|^2 \right). \quad (35)$$

The chemical potential is the functional derivative of the free energy,  $\mu = \delta F/\delta\phi$ . The equilibrium concentration  $\phi_0 = \sqrt{a/b}$  is the minimum of the bulk free energy  $\frac{b}{4}\phi^4 - \frac{a}{2}\phi^2$ . The line tension between the saturated and unsaturated lipid phases  $\sigma$  is related to  $\kappa$  as  $\sigma = 2\sqrt{2}\kappa^{1/2}a^{3/2}b^{-1}/3$  [17, 18]. The interfacial width is given by  $\xi = 1/2\sqrt{\kappa/a}$ . The mobility is related to the lipid diffusivity as  $M = k_B T/(8\pi\eta_m)$ , where  $T$  is the temperature and  $\eta_m$  is the 2D surface membrane viscosity [18]. By dimensional analysis, the characteristic length scales and time scales are  $L_c = \sqrt{\kappa/(2a)}$  and  $t_c = \kappa/(4a^2M)$  respectively. We use the physical properties of lipid membranes to obtain length scales and time scales that match with experimental data. At room temperature (28°C), we estimate lipids have the following properties:  $\phi_0 = 1$ ,  $\sigma = 0.5$  pN,  $\eta_m = 2 \times 10^{-8}$  kg/s, and  $\xi = 50$  nm. The Cahn-Hilliard parameters corresponding to these values are  $M = 2.6 \times 10^{-11}$  m<sup>2</sup>s/kg,  $\kappa = 3.3 \times 10^{-18}$  kg/(m<sup>2</sup>s<sup>2</sup>),  $a = b = 2.9 \times 10^{-4}$  kg/s<sup>2</sup>. For the experiments,  $L_c = 75$  nm and  $t_c = 0.37$  s. In the simulations, the characteristic scales are  $L_c = 0.5$  and  $t_c = 0.25$ . We compare the simulation scales with the experiments to get the following conversion: 1 simulation time unit is 1.5 seconds and the system size of length  $32\pi$  corresponds to 15  $\mu\text{m}$ .

## VI. SUPPLEMENTAL FIGURES

- 
- [1] J. A. Spudich and S. Watt, *Journal of Biological Chemistry* **246**, 4866 (1971).
  - [2] S. MacLean-Fletcher and T. D. Pollard, *Biochemical and Biophysical Research Communications* **96**, 18 (1980).
  - [3] S. S. Margossian and S. Lowey, in *Methods in Enzymology*, Vol. 85 (1982) pp. 55–71.
  - [4] M. I. Angelova and D. S. Dimitrov, *Faraday Discussions of the Chemical Society* **81**, 303 (1986).
  - [5] A. D. Edelstein, M. A. Tsuchida, N. Amodaj, H. Pinkard, R. D. Vale, and N. Stuurman, *Journal of Biological Methods* **1**, e10 (2014).
  - [6] R. Cerbino and V. Trappe, *Physical Review Letters* **100**, 188102 (2008).
  - [7] F. Giavazzi, D. Brogioli, V. Trappe, T. Bellini, and R. Cerbino, *Physical Review E* **80**, 031403 (2009).
  - [8] F. Giavazzi, C. Malinverno, G. Scita, and R. Cerbino, *Frontiers in Physics* **6**, 1 (2018).
  - [9] J. W. Cahn, *The Journal of Chemical Physics* **42**, 93 (1965).
  - [10] J. Toner and Y. Tu, *Physical Review E* **58**, 4828 (1998).
  - [11] L. M. C. Janssen, *Frontiers in Physics* **6** (2018).
  - [12] A. R. Dulaney and J. F. Brady, *Physical Review E* **101**, 052609 (2020).
  - [13] F. J. Sevilla and P. Castro-Villarreal, *Physical Review E* **104**, 064601 (2021).
  - [14] C. Kurzthaler, S. Leitmann, and T. Franosch, *Scientific Reports* **6**, 36702 (2016).
  - [15] Y. Zhao, C. Kurzthaler, N. Zhou, J. Schwarz-Linek, C. Devailly, J. Arlt, J.-D. Huang, W. C. K. Poon, T. Franosch, V. A. Martinez, and J. Tailleur, *Physical Review E* **109**, 014612 (2024).
  - [16] A. J. Bray, A. Cavagna, and R. D. M. Travasso, *Physical Review E* **65**, 016104 (2001).
  - [17] J. W. Cahn and J. E. Hilliard, *The Journal of Chemical Physics* **28**, 258 (1958).
  - [18] B. A. Camley and F. L. H. Brown, *Physical Review Letters* **105**, 148102 (2010).

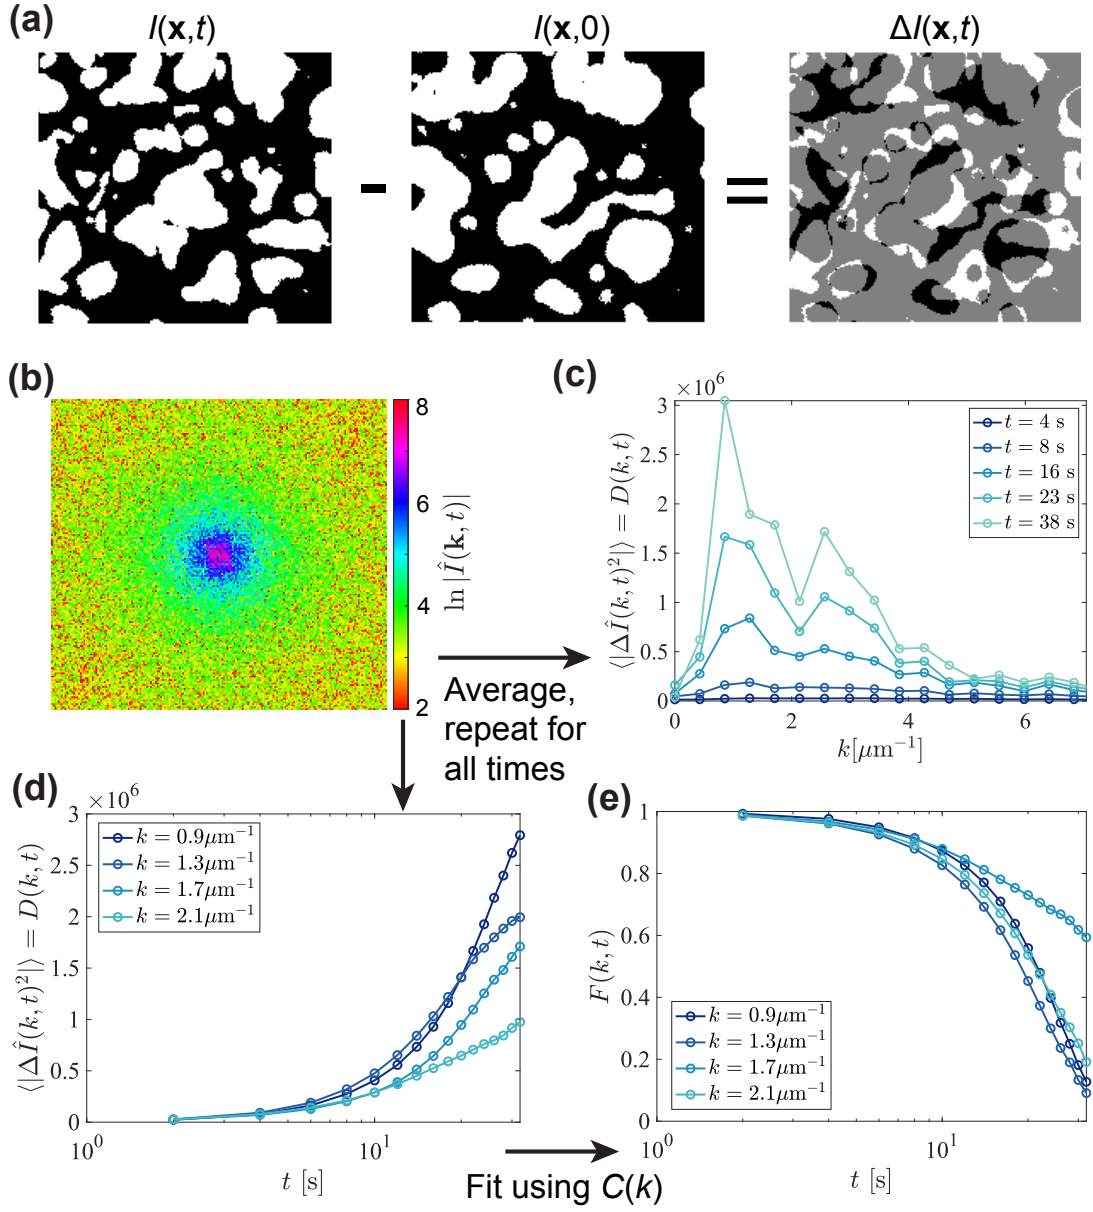

FIG. S1. Example of intermediate scattering function calculation for an active sample. (a) Binarized images of the same sample, separated by lag time  $t$  are subtracted to create a difference image of intensity shift  $\Delta I(\mathbf{x}, t)$ . As the images are binary, three possible values of  $\Delta I$  exist: -1 (black), 0 (gray), and 1 (white). (b) The discrete Fourier transform  $\Delta \hat{I}(\mathbf{x}, t)$  of the difference image is calculated for each pair of images separated by a given  $t$ . Here, we plot the logarithm the Fourier transform of the difference image given in part (a). (c) For all pairs of images separated by a given  $t$ , we average the Fourier transform of the differences and bin the wave vectors, giving the image structure function  $D(k, t)$ . Here  $D(k, t)$  is plotted as a function of wave vector  $k$  for a variety of lag times in an active data set. (d) The image structure function  $D(k, t)$  is plotted as a function of lag time  $t$  for different wave vectors  $k$ . (e) The image structure function  $D(k, t)$  is converted to the intermediate scattering function  $F(k, t)$  using Eq. 6 and the parameter  $C(k)$ , found using the Monte-Carlo methods in Fig. S2.

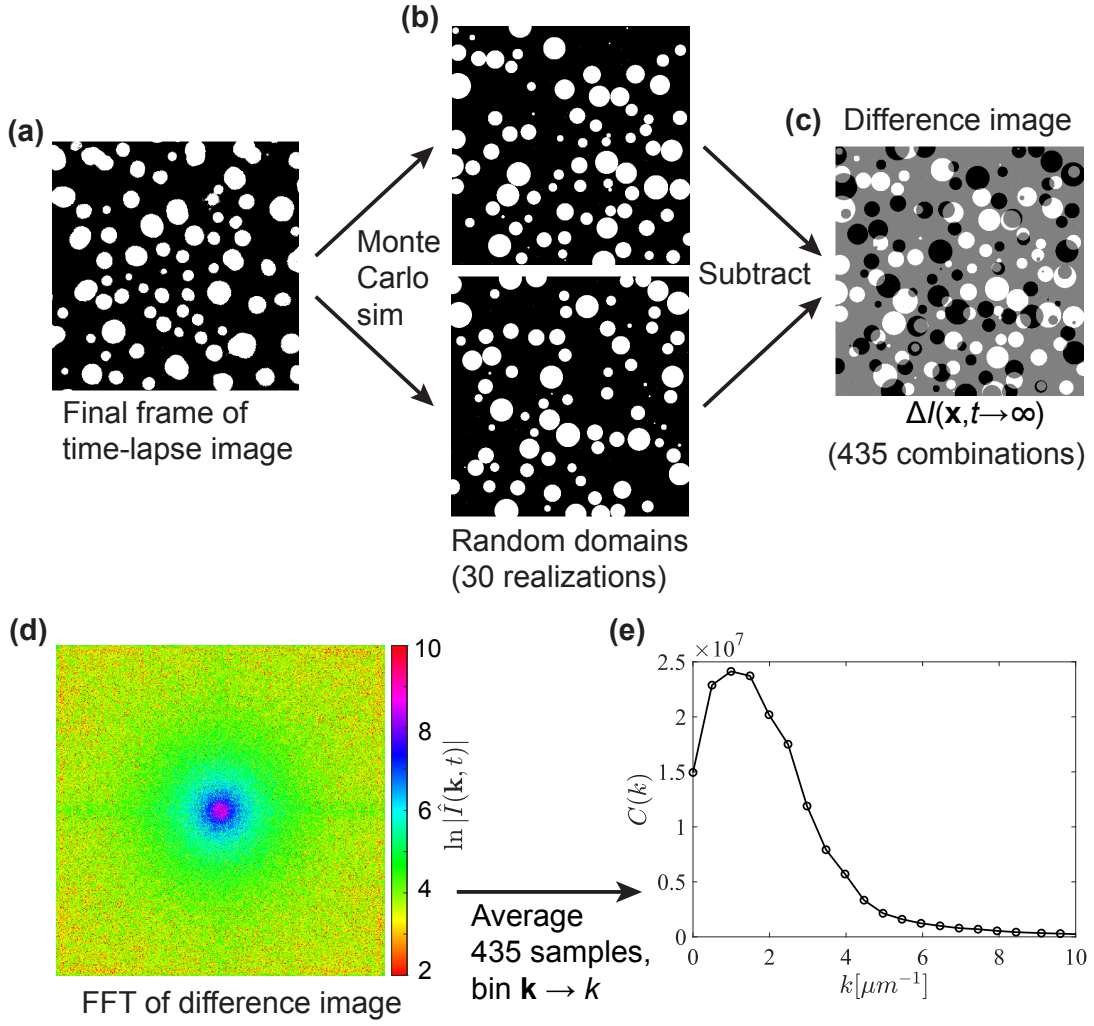

FIG. S2. Graphical representation of the workflow described in Section III A 1 to simulate fully relaxed domains and obtain  $C(k)$  from Eq. 7. (a) The final frame of the experimental time-lapse is binarized. (b) Monte Carlo simulations generate 30 random domain configurations using circles of matching area to the domains in the original experiment, presented here as binary images. (c) The difference is taken between all pairs of binary images (435 in total). As the original images are binary, each pixel in the difference image holds a value of either -1 (black), 0 (gray), or 1 (white). (d) The Fourier transform of each difference image is taken using the fast Fourier transform (FFT) algorithm. (e) The mean square magnitude of the Fourier coefficients in all images is taken according to Eq. 7. The wave vectors are then grouped in  $0.5 \mu\text{m}^{-1}$ -wide bins and averaged, to give the long-time relaxed data  $C(k)$ .  $C(k)$  is ultimately used to find the intermediate scattering function  $F(k, t)$ , as described implicitly in Eq. 6.

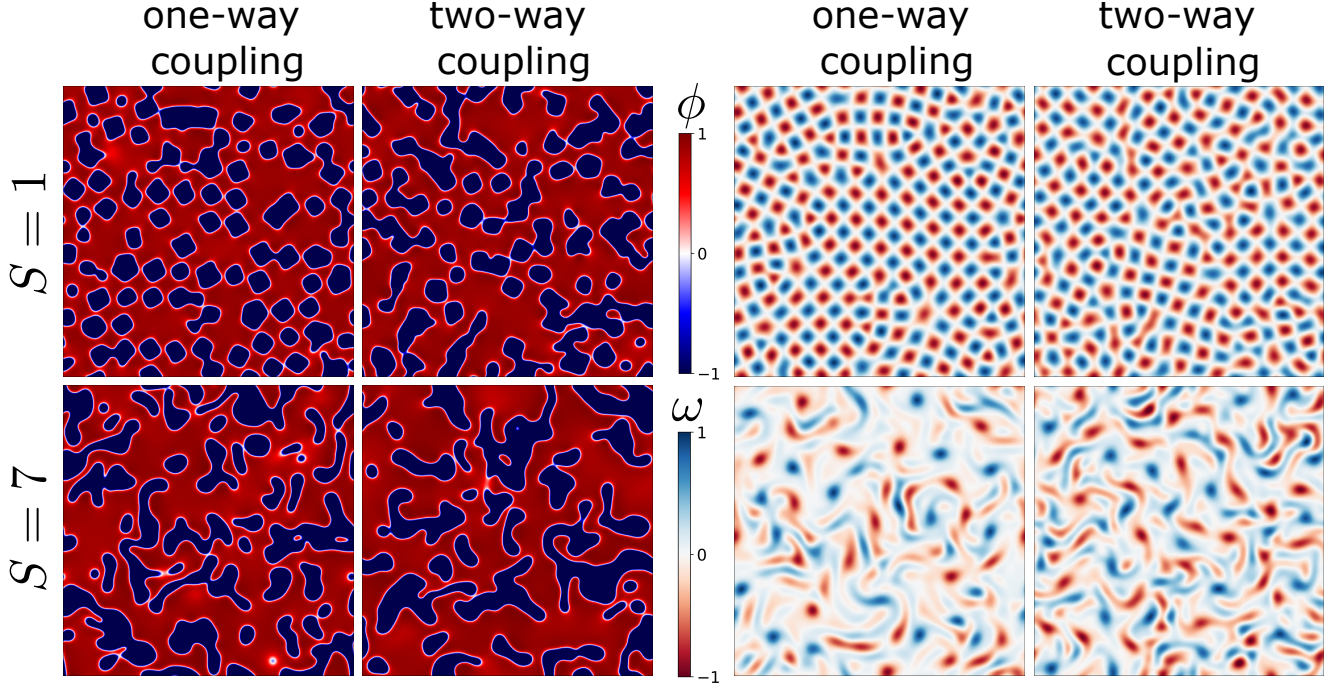

FIG. S3. Numerical simulation snapshots of the concentration order parameter  $\phi$  and vorticity  $\omega = \nabla \times \mathbf{v}$  for  $S = 1, 7$ , with one-way (left) and two-way (right) coupling between  $\phi$  and  $\omega$ . The model parameters used here are  $(M, \kappa, \Gamma_0, \Gamma_2, \alpha, \beta) = (1, 0.25, 1, -1, -0.2, 1)$ .

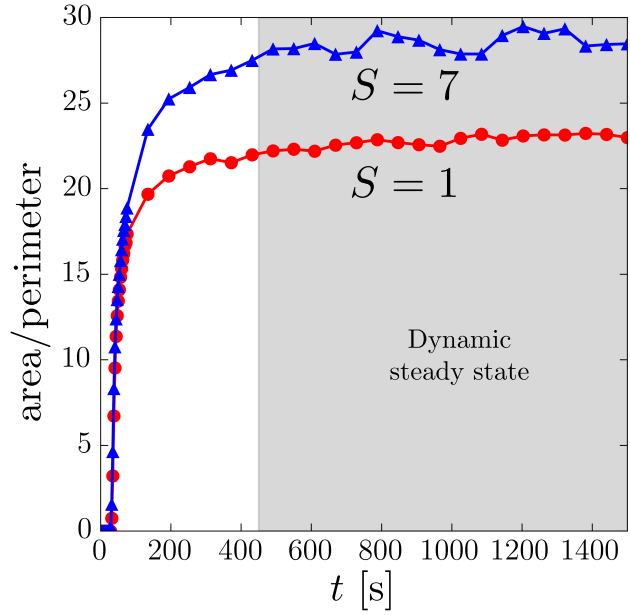

FIG. S4. Evolution of domain size,  $a(t)$ , over time,  $t$ . The ratio of area and perimeter of the domain is the average size of domains. For both  $S = 1, 7$ , the domain size plateaus. We denote the shaded area as the regime where the system reaches a dynamic steady state. In this regime, we calculated the intermediate scattering function [Figs. 2(a, b), 3(b) of main text].

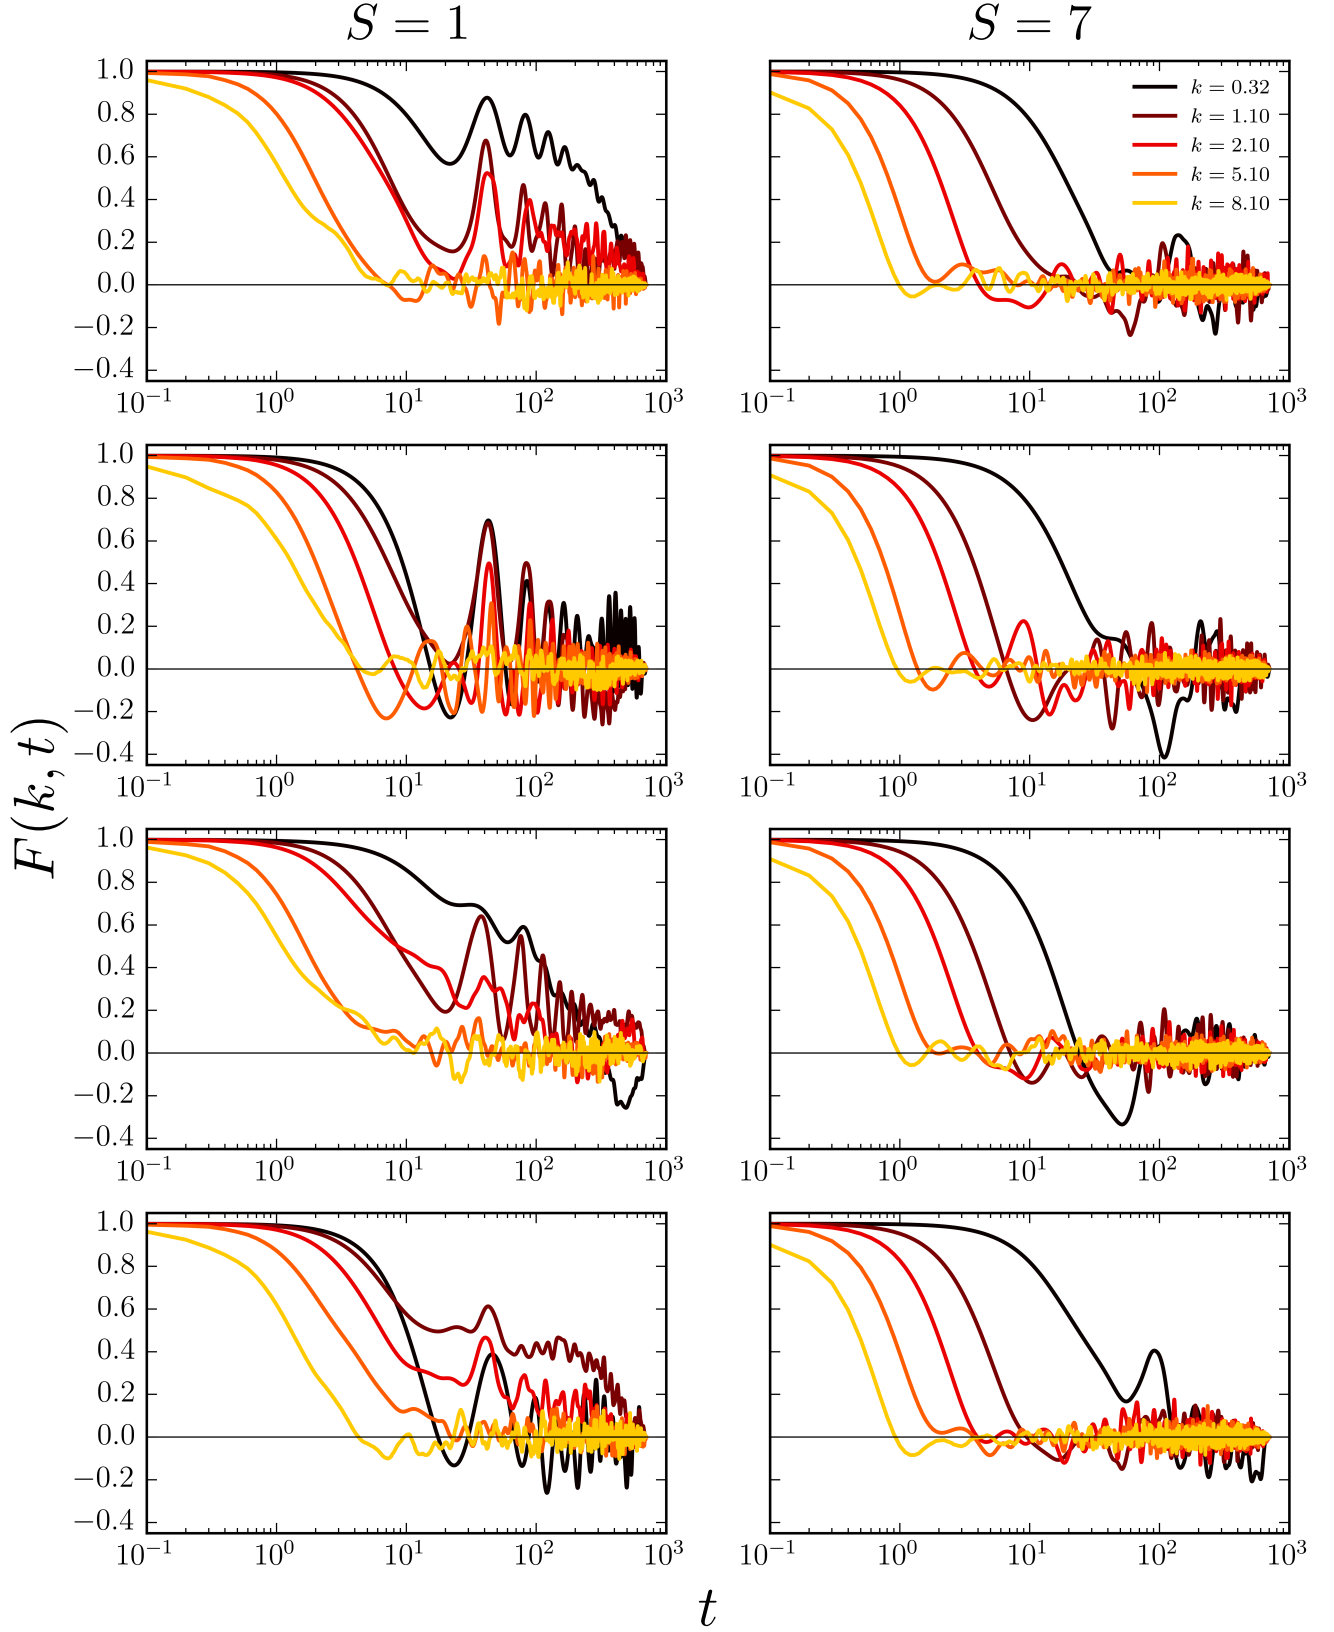

FIG. S5. Intermediate scattering function  $F(k, t)$  is plotted over lag time  $t$  (arbitrary units) for  $S = 1$  (left) and  $S = 7$  (right) for wave vectors  $k = 0.32, 1.10, 2.10, 5.10, 8.10$  (arbitrary units). Each row corresponds to  $F(k, t)$  of a single realization. The Toner Tu equations produce turbulent chaotic flows. So, the evolution of the flows is sensitive to noise in the initial state of the system, causing the relaxation dynamics of each realization to be different.

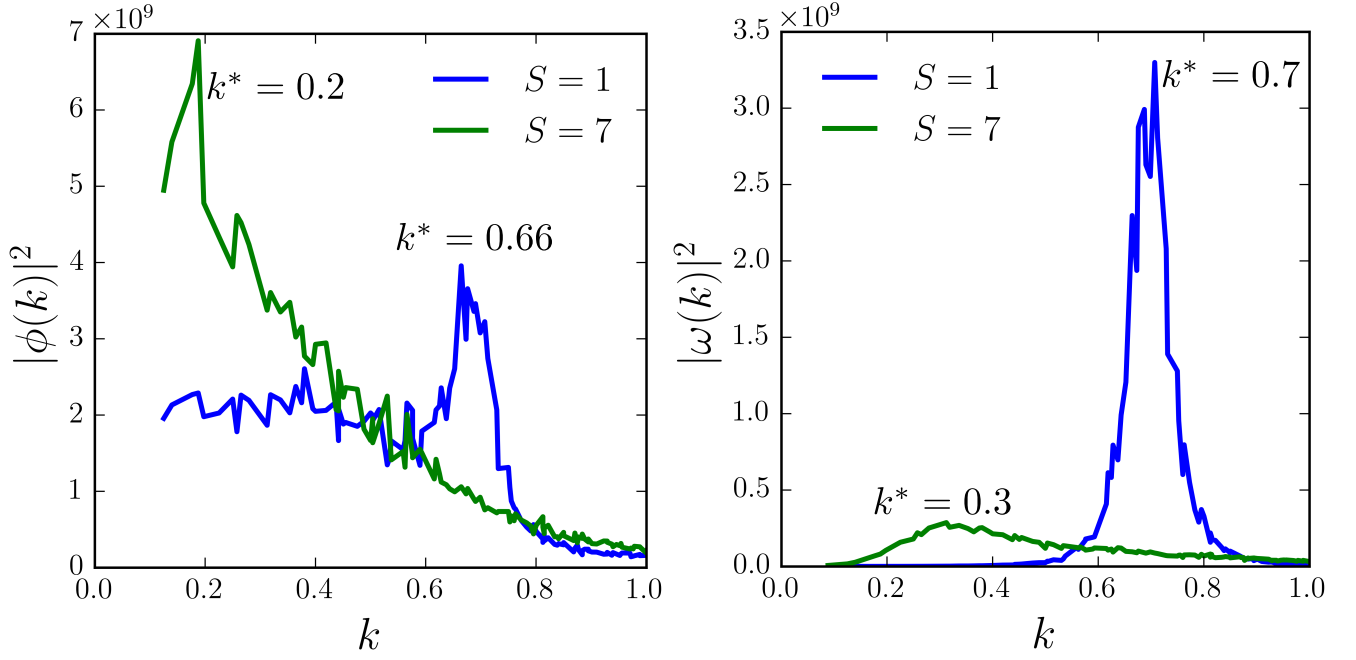

FIG. S6. Static structure factor of the concentration order parameter  $\phi$  and vorticity  $\omega$  at long times is plotted as a function of wave number  $k$  (arbitrary units) for  $S = 1$  (blue) and  $S = 7$  (green). The data is averaged over 30 realizations. The wave number corresponding to the peak of the static structure factor  $k^*$  is approximately the same for  $\phi$  and  $\omega$ .

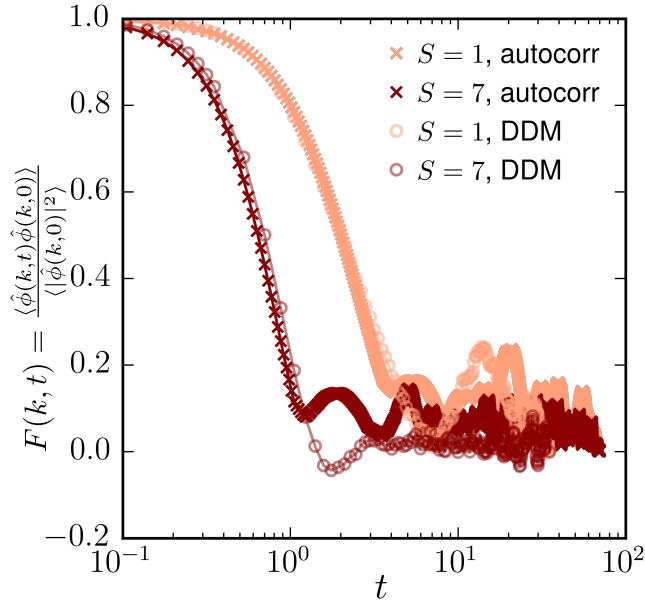

FIG. S7. The intermediate scattering function calculated from direct auto-correlation (labeled as ‘autocorr’ in the figure) is similar to the result obtained from the differential dynamic microscopy (DDM) method. For numerical simulations, we directly compute  $F(k, t)$  as an auto-correlation.

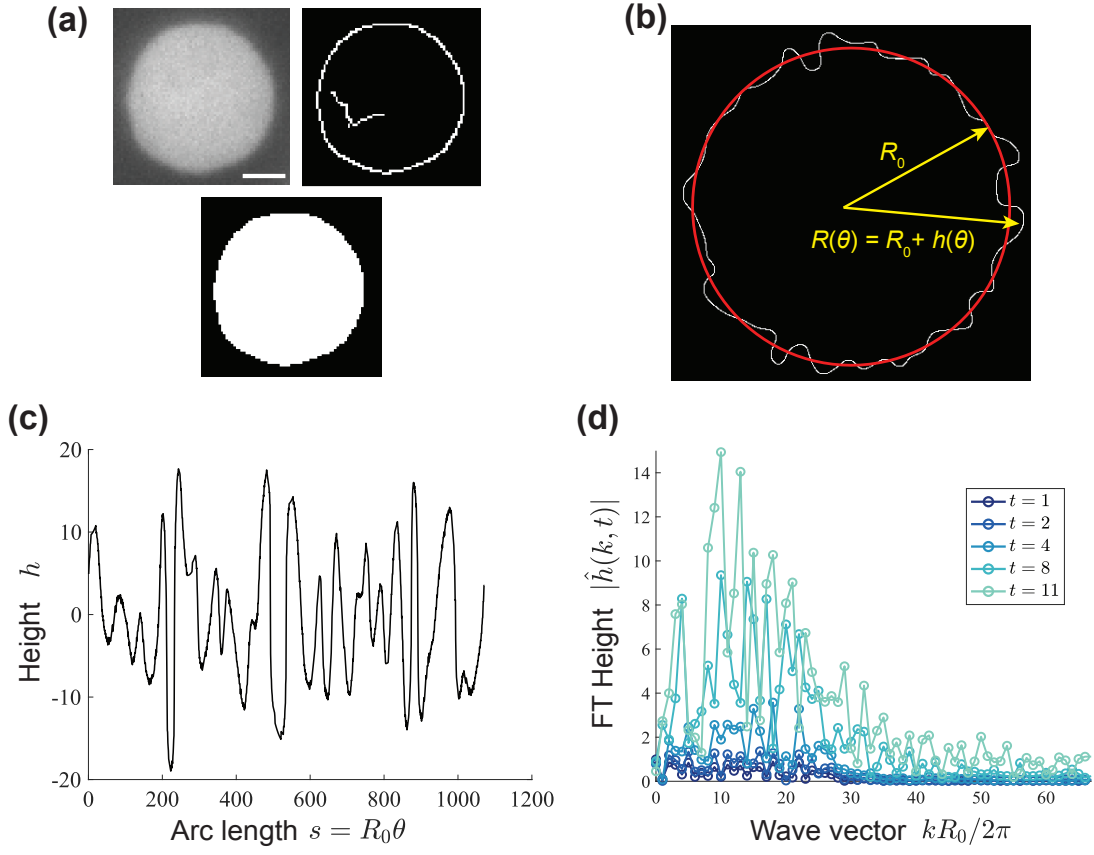

FIG. S8. Analysis of domain interfacial fluctuations. (a) Canny edge detection is used to find the boundary (upper right) of a raw image (upper left). The domain is filled, removing all other artifact edges (bottom). Scale bar is  $2\ \mu\text{m}$ . (b) The edge of a simulated lipid domain is plotted (white), and the distance from each discrete pixel from the center of mass,  $R(\theta)$ , is calculated as a function of the azimuthal angle  $\theta$ . The mean radius  $R_0$  is calculated, and an equivalent circle plotted in red. For each pixel in the domain edge, the deviation from circularity, "height" of the interface  $h(\theta) = R(\theta) - R_0$ , is calculated. (c) Height of the simulated domain in part (b) (in pixel units) is plotted as a function of arc length (also in pixels) of an equivalent circle,  $s = R_0\theta$ . This height fluctuation as a function of arc length is ultimately Fourier transformed. (d) The spatial Fourier transform of height of the simulated domain in part (b),  $\hat{h}(k, t)$  is plotted for multiple frame numbers  $t$ , as a function of dimensionless wave vector magnitude  $k = |\mathbf{k}|$ .

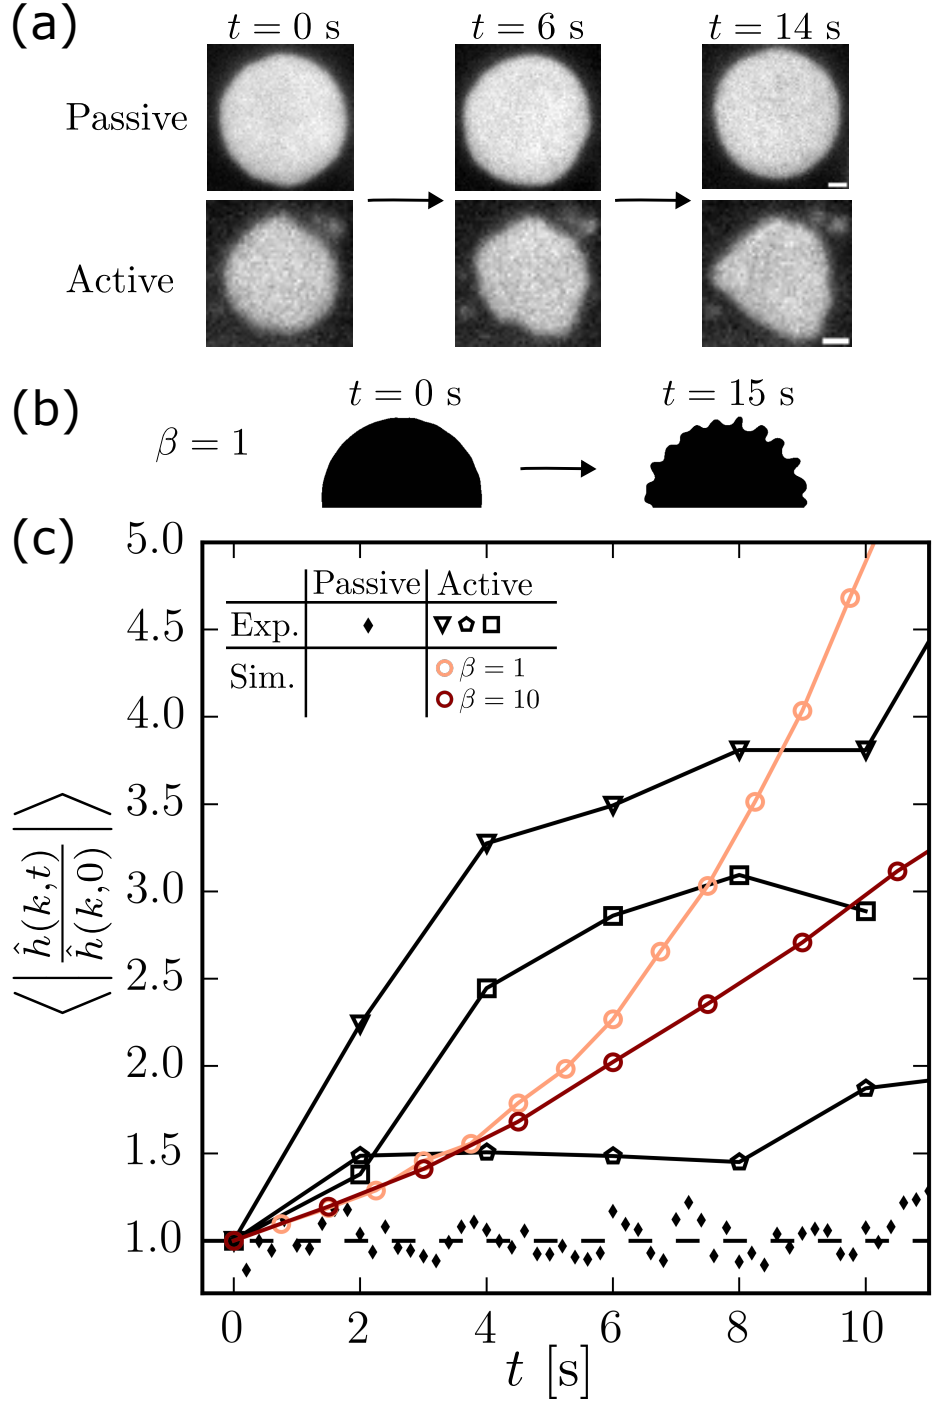

FIG. S9. Interfacial deformations are analyzed with and without the presence of activity. (a) Experiment snapshots of fluctuating passive (top row) and active (bottom row) domains at times  $t = 0$ ,  $6$ ,  $14$  s. (b) Numerical solution snapshots for active domains at  $t = 0$ ,  $15$  s for  $\beta = 1$ . Initially-circular domains are cropped to improve clarity of fluctuations. (c) Fourier-transformed interfacial height  $\hat{h}(k, t)$ , normalized by initial height  $\hat{h}(k, 0)$ , is plotted as a function of time. Experimental data is plotted at a wave vector of  $k \approx 2 \mu\text{m}^{-1}$ . For simulations, the normalized interfacial height spectrum is averaged over all wave vectors. Activity drives the growth of initial perturbations at domain interfaces in both experiments (black open symbols) and simulations (red, salmon). In contrast, thermal fluctuations dampen interfacial perturbations in passive experiments (black diamonds). The  $\beta$  parameter in Eq. 10 is varied to control the speed of the flock, given by  $v_0 = \sqrt{-\alpha/\beta}$ . For high speed flows ( $\beta = 1$ , light red), the interfacial fluctuations grow rapidly. In contrast, the fluctuations grow more slowly for flocks moving at a low speed ( $\beta = 10$ , dark red). The model parameters used here are:  $(M, \kappa, \Gamma_0, \Gamma_2, \alpha, S) = (1, 0.25, -1, 1, -0.2, 7)$ .
